# Supplementary material for: CoCoLM: COmplex COmmonsense Enhanced Language Model with Discourse Relations
Source: arXiv:2012.15643 source file (2022-05-26)
Supplement: Supplementary file 1 [file appendix.tex]

\newcommand\BibTeX{B\textsc{ib}\TeX}

\usepackage[utf8]{inputenc} % allow utf-8 input
\usepackage[T1]{fontenc}    % use 8-bit T1 fonts
\usepackage{hyperref}       % hyperlinks
\usepackage{url}            % simple URL typesetting
\usepackage{booktabs}       % professional-quality tables
\usepackage{amsfonts}       % blackboard math symbols
\usepackage{nicefrac}       % compact symbols for 1/2, etc.
\usepackage{lipsum}
\usepackage{graphicx}
\graphicspath{ {./images/} }

\usepackage{soul}
\usepackage{url}
\usepackage[utf8]{inputenc}
\usepackage[small]{caption}
\usepackage{amsmath}
% \usepackage{amsthm}
\usepackage{booktabs}
\usepackage{algorithm}
\usepackage{algorithmic}
\usepackage[shortlabels]{enumitem}
\usepackage[TABBOTCAP]{subfigure}
\usepackage{multirow}
\usepackage{diagbox}

\newcommand{\ex}[1]{{\sf #1}}

\usepackage{color}

\usepackage{xcolor}
\usepackage{soul}
\newcommand{\hlc}[2][yellow]{{%
    \colorlet{foo}{#1}%
    \sethlcolor{foo}\hl{#2}}%
}



\appendix
\section{Discourse Relation Markers}

\begin{table}[h]
 \centering
 \setlength\tabcolsep{6pt}
 \begin{tabular}{l|c|c}
 \toprule
  Type  &  Relations &  Connectives     \\ \midrule 
     %& en &  fr & zh & ja & it & th & fi & el  \\ \midrule
 \multirow{3}{*}{\begin{minipage}{0.8in}Temporal \end{minipage}}& Precedence  &  before    \\
 & Succession  & after    \\ 
 & Synchronous  & meanwhile     \\ 
 \midrule
 \multirow{3}{*}{\begin{minipage}{0.8in}Casual \end{minipage}}& Reason  & because       \\
 & Result & so      \\
 & Condition  & if  \\ \midrule
 \multirow{4}{*}{\begin{minipage}{0.8in}Others \end{minipage}}& Conjunction  & and       \\
 & Contrast & but      \\
 & Alternative  & or  \\
 & Concession  & although \\
 \bottomrule

 \end{tabular}
 \caption{\label{tab:relation_marker} }  
\end{table}


%\appendix
